# Supplementary material for: Reachability-based Trajectory Design with Neural Implicit Safety Constraints
Source: arXiv:2302.07352 source file (2023-02-14)
Supplement: Supplementary file 1 [file appendix_polyzono.tex]

\section{Definitions of Operations in Tab. \ref{tab:poly_zono_operations}}
\label{app:PZOpDefs}
\jon{comment this out and refer to ARMOUR paper}
This appendix provides definitions for the interval and polynomial zonotope operations given in Tab. \ref{tab:poly_zono_operations}.
% Before proceeding further, note that for vectors $a, b \in \R^3$, we write the cross product $a \times b$ as $a^\times b$, where
% \begin{equation}
%     \label{eq:cross_product_matrix}
%     a^\times= \begin{bmatrix}
%     0 & -a_3 & a_2 \\
%     a_3 & 0 & -a_1 \\
%     -a_2 & a_1 & 0
%     \end{bmatrix}.
% \end{equation}

% \subsection{Polynomial Zonotope Operations}

% First, intervals can be written as polynomial zonotopes.
% Consider the interval $[z] = [\underline{z}, \overline{z}] \subset \mathbb{R}^n$.
% We can convert $[z]$ to a polynomial zonotope $\pz{z}$ using
% \begin{equation}
%     \label{eq:APPint_to_pz}
%     \pz{z} = \frac{\overline{z} + \underline{z}}{2} + \sum_{i = 1}^{n}\frac{\overline{z}_i - \underline{z}_i}{2}x_i,
% \end{equation}
% where $x \in [-1, 1]^n$ is the indeterminate vector.

% Next, we introduce several useful operations for polynomial zonotopes.

% Similar to zonotopes, intervals can also be written as polynomial zonotopes.
% Consider the interval $[z] = [\underline{z}, \overline{z}] \subset \mathbb{R}^n$.
% We can convert $[z]$ to a polynomial zonotope $\pz{z}$ using
% \begin{equation}
%     \label{eq:int_to_pz}
%     \pz{z} = \frac{\overline{z} + \underline{z}}{2} + \sum_{i = 1}^{n}\frac{\overline{z}_i - \underline{z}_i}{2}x_i,
% \end{equation}
% where $x \in [-1, 1]^n$ is the indeterminate vector.

First, the Minkowski Sum of two polynomial zonotopes $\pz{P}_1 \subset \R^n = \PZ{ \pzgi, \pzei, \pzv } $ and $\pz{P}_2 \subset \R^n = \PZ{ h_j, \beta_j, y }$ follows from polynomial addition:
\begin{align}
    \pz{P}_1 \oplus \pz{P}_2 &= \{ z \in \R^n \, \mid \, z = p_1 + p_2, p_1 \in \pz{P}_1, p_2 \in \pz{P}_2 \} \\
     &=
        \left\{
            z \in \R^n \mid z = \sum_{i=0}^{\pzn} \pzgi \pzv ^{\pzei} + \sum_{j=0}^{n_h} h_j y^{\beta_j}
        \right\}. \label{eq:pz_minkowski_sum}
\end{align}
Similarly, we may write the matrix product of two polynomial zonotopes $\pz{P}_1$ and $\pz{P}_2$ when the sizes are compatible (i.e., elements in $\pz{P}_1$ have the same number of columns as elements of $\pz{P}_2$ have rows).
Letting $\pz{P}_1 \subset \R^{n \times m}$ and $\pz{P}_2 \subset \R^{m \times k}$, we obtain $\pz{P}_1 \pz{P}_2 \subset \R^{n \times k}$:
\begin{align}
    \pz{P}_1 \pz{P}_2 &= \{ z \in \R^{n \times k} \, \mid \, z = p_1p_2, p_1 \in \pz{P}_1, p_2 \in \pz{P}_2 \} \\
    &= \left\{
            z \in \R^{n \times k} \, \mid \, z = \sum_{i=0}^{\pzn} \pzgi(\sum_{j=0}^{q} h_j y^{\beta_j}) \pzv ^{\pzei}
        \right\}. \label{eq:pz_multiplication}
\end{align}
When $\pz{P}_1 \subset \R^{n \times n}$ is square, exponentiation $\pz{P}_1^m$ may be performed by multiplying $\pz{P}_1$ by itself $m$ times.

% Furthermore, if $\pz{P}_1 \subset \R^{3}$ and $\pz{P}_2 \subset \R^{3}$, we implement a set-based cross product as matrix multiplication.
% We create $\pz{P}_1^\times \subset \R^{3 \times 3}$ as
% \begin{align}
%     \pz{P}_1^\times = \left\{ A \in \R^{3 \times 3} \, \mid \, A = \sum_{i = 0}^{\pzn}
%         \left[\begin{smallmatrix}
%             0 & -\pzg_{i,3} & \pzg_{i,2} \\ \pzg_{i,3} & 0 & -\pzg_{i,1} \\ -\pzg_{i,2} & \pzg_{i,1} & 0
%         \end{smallmatrix}\right] \pzv ^{\pzei}
%     \right\} \label{eq:pz_cross_product_matrix}
% \end{align}
% where $g_{i, j}$ refers to the $j$\ts{th} element of $g_i$.
% Then, the set-based cross product $\pz{P}_1 \otimes \pz{P}_2 = \pz{P}_1^{\times} \pz{P}_2$ is well-defined. 
We briefly note that the addition and multiplication of a polynomial zonotope with a constant vector or matrix is well-defined if the constant is appropriately sized.
In this case, one constructs a polynomial zonotope with that constant vector or matrix as the center $g_0$ and no other generators, and applies the definitions above.

Both Minkowski summation and  multiplication of polynomial zonotopes can be complicated by the fact that $\pz{P}_1$ and $\pz{P}_2$ may share indeterminates.
For instance, in the examples above, the $i$-th element of $\pzv$ and the $j$-th element of $y$ may represent the same indeterminate.
In practice, polynomial zonotopes can be brought to a \textit{common representation} by only considering unique indeterminates before applying the operations above, as discussed in \cite[Sec. II.a.1]{kochdumper2020sparse}.

Though we have defined several basic operations like addition and multiplication above, it may be desirable to use polynomial zonotopes as inputs to more complicated functions.
One can overapproximate any analytic function evaluated on a polynomial zonotope using a Taylor expansion, which itself can be represented as a polynomial zonotope \cite[Sec 4.1]{althoff2013reachability}\cite[Prop. 13]{kochdumper2020sparse}.
Consider an analytic function $f: \R \to \R$ and $\pz{P}_1 = \PZ{ \pzgi, \pzei, \pzv }$, with each $\pzgi \in \R$.
Then, 
\begin{equation}
    f(\pz{P}_1) = \{ y \in \R \; | \; y = f(z), z \in \pz{P}_1 \}.
\end{equation}
We generate $\pz{P}_2$ such that $f(\pz{P}_1) \subseteq \pz{P}_2$ using a Taylor expansion of degree $d \in \N$, where the error incurred from the finite approximation is overapproximated using a Lagrange remainder.
The method follows the Taylor expansion found in the reachability algorithm in \cite{kochdumper2020sparse}, which builds on previous work on conservative polynomialization found in \cite{althoff2013reachability}.
Recall that the Taylor expansion about a point $c \in \R$ is
\begin{equation}
    f(z) = \sum_{n = 0}^{\infty} \frac{f^{(n)}(c)}{n!} (z - c)^n,
\end{equation}
where $f^{(n)}$ is the $n$\ts{th} derivative of $f$.
Note that the error incurred by a finite Taylor expansion can be bounded using the Lagrange remainder $r$ \cite[7.7]{apostol1991calculus}:
\begin{equation}
    |f(z) - \sum_{n=0}^{d} \frac{f^{(n)}(c)}{n!} (z - c)^n | \leq r,
\end{equation}
where $r$ is given by
\begin{align}
    r &= \frac{M |z - c |^{d+1}}{(d+1)!}, \\
    M &= \underset{\delta \in [c,z]} {\max}( | f^{d+1}(\delta) | ).
\end{align}

For a polynomial zonotope, the infinite dimensional Taylor expansion is given by
\begin{equation}
\label{eq:pz_taylor_inf}
    f(\pz{P}_1) =
    \sum_{n=0}^{\infty}
    \frac{f^{(n)}(c)}{n!} 
    (\pz{P}_1 - c)^n 
\end{equation}
In practice, only a finite Taylor expansion of degree $d \in \N$ can be computed.
Letting $c = \pzg_0$ (i.e., the center of $\pz{P}_1$), and noting that $(z - c) = \sum_{i=1}^{\pzn}\pzgi \pzv ^{\pzei}$ for $z \in \pz{P}_1$, we write
\begin{equation}
\label{eq:pz_taylor_fin}
    \pz{P}_2 \coloneqq
        \left\{ z \in \R \, | \, z \in
            \sum_{n=0}^{d} \left (
            \frac{f^{(n)}(\pzg_0)}{n!} 
            (\sum_{i=1}^{\pzn}\pzgi \pzv ^{\pzei})^n 
            \right )
            \oplus [r]
        \right\}
\end{equation}
% \pat{bleh doesn't quite make sense}
and the Lagrange remainder $[r]$ can be computed using interval arithmetic as
\begin{align}
    [r] &= \frac{[M] [(\pz{P}_1 - c)^{d+1}]}{(d+1)!}, \\ 
    [M] &= f^{(d+1)}([\pz{P}_1])
\end{align}
where $[(\pz{P}_1 - c)^{d+1}] = [\setop{inf}((\pz{P}_1 - c)^{d+1}), \setop{sup}((\pz{P}_1 - c)^{d+1})]$ is an overapproximation of $(\pz{P}_1 - c)^{d+1}$.
Note that $\pz{P}_2$ can be expressed as a polynomial zonotope because all terms in the summation are polynomials of $\pzv$, and the interval $[r]$ can be expressed as a polynomial zonotope.
Just as we denote polynomial zonotopes using bold symbols, we denote the polynomial zonotope overapproximation of a function evaluated on a zonotope using bold symbols (\emph{i.e.}, $\pz{f}(\pz{P}_1)$ is the polynomial zonotope over approximation of $f$ applied to $\pz{P}$). 
Note the usual order of operations for addition, multiplication and exponentiation apply for polynomial zonotope operations as well.
Table \ref{tab:poly_zono_operations} summarizes these operations.
Note as described in the table these operations can either be computed exactly or in an overapproximative fashion using polynomial zonotopes.

The operations defined above (multiplication in particular) increases the number of generators required to represent a polynomial zonotope, therefore increasing the memory required to store a polynomial zonotope.
In practice, successively applying these operations can become computationally intractable.
To combat this computational burden, we define a \defemph{reduce} operation for a polynomial zonotope.
The reduce operation generates overapproximations of polynomial zonotopes through using fewer generators.
If a polynomial zonotope $\pz{P} \subset \R^n$ has $\pzn$ terms, but a maximum of $q$ terms are desired, excess terms can be overapproximated by an interval:
\begin{align}
    \label{eq:pz_reduce}
    \setop{reduce}(\pz{P}, n_h) = \left\{ z \in \R^n \, \mid \, z \in \sum_{i=0}^{n_h-n} \pzgi \pzv ^{\pzei} \oplus [-b, b]\right\}
\end{align}
where $b_j$ is equal to $\sum_{i=n_h-n+1}^{\pzn} | g_{i,j} |$ where $g_{i,j}$ is the $j$\ts{th} element of $\pzgi$.
This means that the last $\pzn - n_h - n + 1$ terms are overapproximated by an $n$-dimensional hyperbox represented by an interval.
This interval can be expressed as a polynomial zonotope as in \eqref{eq:int_to_pz}, and so the output of $\setop{reduce}(\pz{P}, q)$ is itself a polynomial zonotope.
% \pat{this was not quite written right... sum is over the $j$-th dimension}
Notice that $\setop{reduce}(\pz{P}, q)$ always overapproximates $\pz{P}$, i.e. $\pz{P} \subseteq \setop{reduce}(\pz{P}, q)$ \cite[Prop. 16]{kochdumper2020sparse}.
One can reorder the terms of the polynomial zonotope such that only certain desirable terms are replaced by intervals, e.g. to produce a tighter overapproximation.
