# Supplementary material for: Reachability-based Trajectory Design with Neural Implicit Safety Constraints
Source: arXiv:2302.07352 source file (2023-02-14)
Supplement: Supplementary file 2 [file appendix.tex]

\section{Proof of Lem. \ref{lem:zono_positive_distance}}
\label{app:pz_distance_proof}

\begin{proof}
The distance between $Z_1$ and $Z_2$ is given by
\begin{align}
    &d(Z_1,Z_2) = \underset{p_1,p_2}{min} &&||p_1-p_2|| \\
    &&& p_i \in Z_i \qquad i=1,2 
\end{align}
By definition 12, 
\begin{align}
    & p_i\in Z_i \Longleftrightarrow p_i = c_i + G_i\,\beta_{i}, \;||\beta_{i}||_{\infty}\leq1. 
\end{align}
Then, by denoting $G_{buf}=\lbrack G_1\;G_2 \rbrack$ and $\beta_{buf}^\top=\lbrack -\beta_1^\top\;\beta_2^\top \rbrack$,
\begin{align}
    &\underset{p_1,p_2}{\min} &&||p_1-p_2|| \\
    &&& p_i \in Z_i \qquad i=1,2 \\
    &=\underset{\beta_1,\beta_2}{\min} &&||(c_1 + G_1\,\beta_{1})-(c_2 + G_2\,\beta_{2})|| \\
    &&& ||\beta_{i}||_{\infty}\leq1 \qquad i=1,2 \\
    &=\underset{\beta_{buf}}{\min} &&||c_1-(c_2 + G_{buf}\,\beta_{buf})|| \\
    &&& ||\beta_{buf}||_{\infty}\leq1\\
    &=\underset{p}{\min} &&||c_1-p|| \\
    &&& p \in Z_{2,buf}\\
    &=d(c_1,Z_{2,buf})
\end{align}
Therefore, $d(Z_1, Z_2) = d(c_1; Z_{2,buf})$.
\end{proof}
